# Supplementary material for: Bayesian method for causal inference in spatially-correlated multivariate time series
Source: arXiv:1801.06282 ancillary file (2018-03-12)
Supplement: Supplementary file 1 [file Supplementary-material.pdf]

# Supplement to ‘Bayesian method for causal inference in spatially-correlated multivariate time series’

Bo Ning<sup>\*</sup>, Subhashis Ghosal<sup>\*</sup> and Jewell Thomas<sup>†‡</sup>

**MSC 2010 subject classifications:** 62F15.

**Keywords:** Advertising campaign, Bayesian variable selection, causal inference, graphical model, stationarity, time series.

The supplement contains five sections: Section 1 provides the details of the two-stage algorithm. Section 2 gives the details on the derivation of our revised EMVS algorithm. Section 3 provides graphical and tabular representations of the results of the new method to infer causality using the univariate model. Section 4 provides model checking results. Section 5 describes the Kalman filter and backward smoothing algorithm.

## 1 The two-stage algorithm

The two-stage algorithm is proposed as follows. In Stage 1, we estimate the sparse regression parameter  $\hat{\beta}$ . In Stage 2, we sample the parameters in the model (except  $\beta$ ) using the MCMC algorithm, which is described in Section 4 of the paper. In below, we provide the details of our algorithm.

### 1.1 Estimating the sparse regression parameter

If we let  $\mathbf{Y}_t^* = \mathbf{Y}_t - \mathbb{E}(\mathbf{Y}_t)$ ,  $\mathbf{X}_t^* = \mathbf{X}_t - \mathbb{E}(\mathbf{X}_t)$  and  $\alpha_t^* = \alpha_t - \mathbb{E}(\alpha_t)$ , then we have

$$\begin{aligned}\mathbf{Y}_t^* &= \mathbf{z}\alpha_t^* + \mathbf{X}_t^*\beta + \epsilon_t, \\ \alpha_{t+1}^* &= \mathbf{T}\alpha_t^* + \mathbf{R}\eta_t.\end{aligned}\tag{1.1}$$

Recall that  $\epsilon_t \sim \mathcal{N}(\mathbf{0}, \Sigma)$  and  $\eta_t \sim \mathcal{N}(\mathbf{0}, \mathbf{Q})$  are i.i.d. random errors.

The joint posterior distribution for parameters in this model can be written as

$$\begin{aligned}\pi(\alpha_{1:T}^*, \beta, \gamma, \theta, \Phi, \Sigma, \mathbf{Q} \mid \mathbf{Y}_t^*, \mathbf{X}_t^*) \\ \propto \prod_{t=1}^T f(\mathbf{Y}_t^* \mid \mathbf{X}_t^*, \alpha_t^*, \beta, \Sigma) \prod_{t=2}^T f(\alpha_t^* \mid \alpha_{t-1}^*, \Phi, \mathbf{Q}) \pi(\alpha_1^*) \\ \times \pi(\beta \mid \gamma) \pi(\gamma \mid \theta) \pi(\theta) \pi(\text{vec}(\Phi)) \pi(\Sigma^{-1} \mid \nu, \mathbf{H}) \\ \times \pi(\Sigma_u^{-1} \mid k_1, \nu, \mathbf{H}) \pi(\Sigma_v^{-1} \mid k_2, \nu, \mathbf{H}) \pi(\Sigma_w^{-1} \mid k_3, \nu, \mathbf{H}).\end{aligned}\tag{1.2}$$

<sup>\*</sup>Department of Statistics, North Carolina State University, 2501 Founders Drive, Raleigh, North Carolina 27695, USA. [bning@ncsu.edu](mailto:bning@ncsu.edu), [sghosal@ncsu.edu](mailto:sghosal@ncsu.edu)

<sup>†</sup>Department of English & Comparative Literature, The University of North Carolina at Chapel Hill, CB #3520 Greenlaw Hall, Chapel Hill, North Carolina 27599, USA. [jewellt@live.unc.edu](mailto:jewellt@live.unc.edu)

<sup>‡</sup>Jewell Thomas is a former Staff Data Scientist at MaxPoint Interactive Inc., 3020 Carrington Mill Blvd, Morrisville, North Carolina 27560, USA.

To obtain  $\hat{\beta}$ , we use the revised EMVS algorithm, which will be described in below, and use the priors for almost all the parameters except for  $\Phi$ . Since  $\beta$  is the only parameter we are interested in here, to reduce the complexity of deriving the expression appearing in the EMVS algorithm, we consider a conjugate prior for  $\Phi$ :  $\text{vec}(\Phi) \sim \mathcal{N}(\mathbf{0}, 0.1 \times \mathbf{I}_{n^2})$ . In the simulation study, we show that the choice of the prior for  $\Phi$  is not influential. The details of the revised EMVS algorithm are provided in the supplementary material.

Our EMVS algorithm indirectly maximize the posterior by iteratively maximizing the object function:

$$\begin{aligned} \mathcal{Q}(\beta, \theta, \Phi, \Sigma, \mathbf{Q} \mid \beta^{(k)}, \theta^{(k)}, \Phi^{(k)}, \Sigma^{(k)}, \mathbf{Q}^{(k)}) \\ = C + \mathcal{Q}_1(\beta, \Phi, \Sigma, \mathbf{Q} \mid \beta^{(k)}, \theta^{(k)}, \Phi^{(k)}, \Sigma^{(k)}, \mathbf{Q}^{(k)}) + \mathcal{Q}_2(\theta \mid \beta^{(k)}, \theta^{(k)}), \end{aligned}$$

where  $C$  is a constant,

$$\begin{aligned} \mathcal{Q}_1(\beta, \Phi, \Sigma, \mathbf{Q} \mid \beta^{(k)}, \theta^{(k)}, \Phi^{(k)}, \Sigma^{(k)}, \mathbf{Q}^{(k)}) \\ = -\frac{1}{2} \sum_{t=1}^T \mathbb{E}_{\alpha_{1:T}^*} \left[ (\mathbf{Y}_t^* - \mathbf{X}_t^* \beta - \mathbf{z} \alpha_t^*)' \Sigma^{-1} (\mathbf{Y}_t^* - \mathbf{X}_t^* \beta - \mathbf{z} \alpha_t^*) \right] \\ - \frac{1}{2} \sum_{t=1}^{T-1} \mathbb{E}_{\alpha_{1:T}^*} \left[ (\alpha_{t+1}^* - \mathbf{T} \alpha_t^*)' \mathbf{R} \mathbf{Q}^{-1} \mathbf{R}' (\alpha_{t+1}^* - \mathbf{T} \alpha_t^*) \right] - \frac{1}{2} \alpha_1^{*'} \alpha_1^* \\ + \frac{T + \nu - 2}{2} \log |\Sigma^{-1}| + \frac{T + \nu - 3}{2} \left( \log |\Sigma_u^{-1}| + \log |\Sigma_v^{-1}| + \log |\Sigma_w^{-1}| \right) \\ - \frac{1}{2} \left( \text{Tr}(\mathbf{H} \Sigma^{-1}) + \text{Tr}(k_1^2(n+1) \mathbf{H} \Sigma_u^{-1}) + \text{Tr}(k_2^2(n+1) \mathbf{H} \Sigma_v^{-1}) + \text{Tr}(k_3^2(n+1) \mathbf{H} \Sigma_w^{-1}) \right) \\ - \frac{1}{2 \times 0.1} \text{vec}(\Phi)' \text{vec}(\Phi) - \sum_{i=1}^p \mathbb{E}_{\gamma_i} \left[ \log(v_0(1 - \gamma_i) + v_1 \gamma_i) \right] \\ - \frac{1}{2} \sum_{i=1}^p \beta_i^2 \mathbb{E}_{\gamma_i} \left[ \frac{1}{v_0(1 - \gamma_i) + v_1 \gamma_i} \right], \end{aligned}$$

and

$$\begin{aligned} \mathcal{Q}_2(\theta \mid \beta^{(k)}, \theta^{(k)}) \\ = \sum_{i=1}^p \log \left( \frac{\theta}{1 - \theta} \right) \mathbb{E}_{\gamma_i}(\gamma_i) + (\zeta_1 - 1) \log \theta + (p + \zeta_2 - 1) \log(1 - \theta). \end{aligned}$$

A more detailed derivation of  $\mathcal{Q}_1(\beta, \Phi, \Sigma, \mathbf{Q} \mid \beta^{(k)}, \theta^{(k)}, \Phi^{(k)}, \Sigma^{(k)}, \mathbf{Q}^{(k)})$  and  $\mathcal{Q}_2(\theta \mid \beta^{(k)}, \theta^{(k)})$  are given in Section 2.

After obtaining  $\hat{\beta}$ , we deduct  $\mathbf{X}_t \hat{\beta}$  from  $\mathbf{Y}_t$  and denote the new data as  $\tilde{\mathbf{Y}}_t$ . We then work with the following model in the MCMC step,

$$\begin{aligned} \tilde{\mathbf{Y}}_t &= \mathbf{z} \alpha_t + \epsilon_t, \\ \alpha_{t+1} &= \mathbf{c} + \mathbf{T} \alpha_t + \mathbf{R} \eta_t. \end{aligned} \tag{1.3}$$

The following sub-sections describe sampling techniques for sampling parameters in this model.

## 1.2 Sampling the time-varying parameters

From (1.3), the posterior distribution of  $\alpha_{1:T}$  can be expressed as

$$\pi(\alpha_{1:T}|\boldsymbol{\vartheta}, \tilde{\mathbf{Y}}_t) \propto \prod_{t=1}^T p(\tilde{\mathbf{Y}}_t|\alpha_t, \boldsymbol{\vartheta}) \prod_{t=2}^T p(\alpha_t|\alpha_{t-1}, \boldsymbol{\vartheta}) \pi(\alpha_1) \quad (1.4)$$

with each density being a multivariate normal distribution; here  $\boldsymbol{\vartheta}$  stands for all the parameters in the model excluding  $\alpha_{1:T}$ . To sample  $\alpha_{1:T}$ , we apply the Kalman-filter and simulation smoother algorithm (Durbin and Koopman, 2012, 2002). Recall  $\alpha_1 \sim \mathcal{N}(\mathbf{a}, \mathbf{P})$ . To choose a definite prior for  $\alpha_1$ , we proceed as follows: if  $\alpha_{1:T}$  follows a nonstationary stochastic process, we choose a diffuse prior for  $\alpha_1$ , that is we let  $\mathbf{a} = \mathbf{0}$  and  $\mathbf{P}$  be a diagonal matrix with large diagonal elements. If  $\tau_{1:T}$  is restricted to be stationary, then the component of  $\alpha_1$  corresponding to  $\tau_1$  needs to have a prior distribution with a smaller variance. Under some circumstances, one can estimate the values for the variances using classical methods by treating parameters as time-invariant in a given training datasets (Primiceri, 2005). But here  $\tau_t$  is a latent variable standing for the trend and thus is not estimable. However, we found that the resulting procedure is not sensitive to the choice of values of variance. For example, we can choose the covariance matrix of  $\tau_t$  to be the identity matrix.

## 1.3 Sampling the stationarity constraint parameters $\mathbf{D}$ and $\Phi$

Given the priors described in Section 3 of the paper, we sample the parameters from their posterior distributions using a Metropolis-Hastings algorithm. We choose the proposal density for each parameter to be a normal distribution centered at the value of its latest MCMC draw and variance to be a small number, say 0.1.

One can choose to update  $n^2 + 1$  parameters one by one. However, when  $n$  is large, it is more efficient to update them in blocks. One may choose the block knots to be either fixed or stochastic. For stochastic knots, one may use the method introduced by Shephard and Pitt (1997).

Given a current draw for  $\Phi$ , by using the prior  $\mathcal{N}(\mathbf{0}, \mathbf{I}_n)$ ,  $\mathbf{D}$  can be sampled from its posterior given by

$$\pi(\mathbf{D}|\Phi, \tau_{1:T}) \sim \mathcal{N}(\boldsymbol{\mu}_D, \mathbf{V}_D), \quad (1.5)$$

with

$$\begin{aligned} \mathbf{V}_D &= [(T-1)(\mathbf{I}_n - \Phi)' \Sigma_v^{-1} (\mathbf{I}_n - \Phi) + \mathbf{I}_n]^{-1}, \\ \boldsymbol{\mu}_D &= \mathbf{V}_D [(\mathbf{I}_n - \Phi)' \Sigma_v^{-1} \sum_{t=1}^{T-1} (\tau_{t+1} - \Phi \tau_t)]. \end{aligned}$$

## 1.4 Sampling the covariance matrices of the residuals

The residual error terms are both multivariate normal with precision matrices having the same sparsity structure. In the following we derive the posterior of  $\Sigma^{-1}$ ; the posteriors for  $\Sigma_u^{-1}$ ,  $\Sigma_v^{-1}$  and  $\Sigma_w^{-1}$  can be derived in a similar way. We summarize these parameters in Table 1.

We impose sparsity on  $\Sigma^{-1}$  to reduce the number of parameters needed to be estimated. The sparsity structure is a pre-determined matrix of zeros and ones which assumes that two responses are conditionally independent if the corresponding entry is 0. In Bayesian analysis, sparsity on an inverse covariance matrix is often imposed through a  $\mathcal{G}$ -Wishart prior (Dawid and Lauritzen, 1993; Roverato, 2000, 2002). Given a sparsity structure  $\mathcal{G}$ , the prior  $W_{\mathcal{G}}(\nu, \mathbf{H})$  has the expression

$$\pi(\Sigma^{-1}|\mathcal{G}) = I_{\mathcal{G}}(\nu, \mathbf{H}) |\Sigma^{-1}|^{(\nu-2)/2} \exp\{-\frac{1}{2}\text{tr}(\mathbf{H}\Sigma^{-1})\} \mathbb{1}_{\{\Sigma^{-1} \in M^+(\mathcal{G})\}}, \quad (1.6)$$

where the normalizing constant  $I_{\mathcal{G}}(\nu, \mathbf{H})$  for a decomposable graph is given by

$$I_{\mathcal{G}}(\nu, \mathbf{H}) = \int |\Sigma^{-1}|^{(\nu-2)/2} \exp\{-\frac{1}{2}\text{tr}(\mathbf{H}\Sigma^{-1})\} \mathbb{1}_{\{\Sigma^{-1} \in M^+(\mathcal{G})\}} d\Sigma^{-1}; \quad (1.7)$$

here  $\nu > n-1$  is the degree of freedom,  $\mathbf{H}$  is an  $n \times n$  symmetric positive definite matrix,  $M^+(\mathcal{G})$  is the cone of the symmetric positive definite matrix  $\Sigma^{-1}$  based on the graphical structure  $\mathcal{G}$ . We allow  $\mathcal{G}$  to be either decomposable or non-decomposable and use the BDgraph package in the R library for computation, which uses explicit expression for the normalizing constant in (1.7) if the graph is decomposable and uses the BDMCMC algorithm (Mohammadi and Wit, 2015) if the graph is non-decomposable.

Table 1: Parameters of the posterior densities of  $\Sigma^{-1}$ ,  $\Sigma_u^{-1}$ ,  $\Sigma_v^{-1}$ ,  $\Sigma_w^{-1}$ .

| Parameters      | DF            | Scale matrix                                                                                                                                                                                                  |
|-----------------|---------------|---------------------------------------------------------------------------------------------------------------------------------------------------------------------------------------------------------------|
| $\Sigma^{-1}$   | $T + \nu$     | $\sum_{t=1}^T (\tilde{\mathbf{Y}}_t - \mathbf{z}_t \boldsymbol{\alpha}_t)(\tilde{\mathbf{Y}}_t - \mathbf{z}_t \boldsymbol{\alpha}_t)' + \mathbf{H}$                                                           |
| $\Sigma_u^{-1}$ | $T + \nu - 1$ | $\sum_{t=1}^{T-1} (\boldsymbol{\mu}_{t+1} - \boldsymbol{\mu}_t - \boldsymbol{\tau}_t)(\boldsymbol{\mu}_{t+1} - \boldsymbol{\mu}_t - \boldsymbol{\tau}_t)' + k_1^2(n+1)\mathbf{H}$                             |
| $\Sigma_v^{-1}$ | $T + \nu - 1$ | $\sum_{t=1}^{T-1} (\tilde{\boldsymbol{\tau}}_{t+1} - \boldsymbol{\Phi} \tilde{\boldsymbol{\tau}}_t)(\tilde{\boldsymbol{\tau}}_{t+1} - \boldsymbol{\Phi} \tilde{\boldsymbol{\tau}}_t)' + k_2^2(n+1)\mathbf{H}$ |
| $\Sigma_w^{-1}$ | $T + \nu - 1$ | $\sum_{t=1}^{T-1} (\boldsymbol{\delta}_{t+1} + \sum_{j=0}^{S-2} \boldsymbol{\delta}_{t-j})(\boldsymbol{\delta}_{t+1} + \sum_{j=0}^{S-2} \boldsymbol{\delta}_{t-j})' + k_3^2(n+1)\mathbf{H}$                   |

## 2 Deriving the revised EMVS algorithm

In this section, we provide the details on deriving the revised EMVS algorithm. The algorithm contains two steps: the E-step (the expectation step) and the M-step (the maximization step).

### • E-step

The expectation of  $\boldsymbol{\alpha}_t^*$ ,  $\boldsymbol{\alpha}_t^* \boldsymbol{\alpha}_t^{*'}'$  and  $\boldsymbol{\alpha}_t^* \boldsymbol{\alpha}_{t-1}^{*'}'$  respect to  $\boldsymbol{\alpha}_{1:T}^*|\cdot$  can be estimated using the KFBS algorithm (see details in Section 5).

The term  $\mathbb{E}_{\gamma|\cdot}[\log(v_0(1-\gamma_i) + v_1\gamma_i)]$  is a constant when conditioned on the parameters  $\beta^{(k)}, v_0, v_1$ .

Let  $a_i^{*(k)} = \mathbb{E}_{\gamma|\cdot}[\frac{1}{v_0(1-\gamma_i) + v_1\gamma_i}]$ , because  $\gamma_i$  is a binary variable,

$$a_i^{*(k)} = \mathbb{E}_{\gamma|\cdot}[\frac{1}{v_0(1-\gamma_i) + v_1\gamma_i}] = \frac{\mathbb{E}_{\gamma|\cdot}(1-\gamma_i)}{v_0} + \frac{\mathbb{E}_{\gamma|\cdot}(\gamma_i)}{v_1}.$$

Denote  $w_i^{(k)} = \mathbb{E}_{\gamma|\cdot}(\gamma_i)$ , then

$$w_i^{(k)} = \mathbb{E}_{\gamma|\cdot}(\gamma_i) = P(\gamma_i = 1 | \beta^{(k)}, \theta^{(k)}) = \frac{g_{1i}^{(k)}}{g_{1i}^{(k)} + g_{2i}^{(k)}},$$

where  $g_{1i}^{(k)} = \pi(\beta_i^{(k)} | v_0, v_1, \gamma_i = 1)P(\gamma_i = 1 | \theta^{(k)})$  and  $g_{2i}^{(k)} = \pi(\beta_i^{(k)} | v_0, v_1, \gamma_i = 0)P(\gamma_i = 0 | \theta^{(k)})$ . Based on the prior in Section 3,  $g_{1i}^{(k)}$  and  $g_{2i}^{(k)}$  can be written as  $g_{1i}^{(k)} = \pi(\beta_i^{(k)} | v_0, v_1, \gamma_i = 1)\theta^{(k)}$  and  $g_{2i}^{(k)} = \pi(\beta_i^{(k)} | v_0, v_1, \gamma_i = 0)(1 - \theta^{(k)})$ .

If using DAEMVS algorithm with parameter  $s$ , then

$$w_i^{(k)} = \frac{(g_{1i}^{(k)})^s}{(g_{1i}^{(k)})^s + (g_{2i}^{(k)})^s}.$$

To summarize, in the  $k$ -th E-step, we find

$$\begin{aligned} & \mathcal{Q}(\beta, \theta, \Phi, \Sigma, Q | \beta^{(k)}, \theta^{(k)}, \Phi^{(k)}, \Sigma^{(k)}, Q^{(k)}) \\ &= \mathbb{E}_{(\alpha_{1:T}^*, \gamma)|\cdot}[\log \pi(\alpha_{1:T}^*, \beta, \gamma, \theta, \Phi, \Sigma, Q | Y_t^*, X_t^*) | \beta^{(k)}, \theta^{(k)}, \Phi^{(k)}, \Sigma^{(k)}, Q^{(k)}], \end{aligned} \quad (2.1)$$

where  $\mathbb{E}_{(\alpha_{1:T}^*, \gamma)|\cdot}(\cdot)$  denotes the conditional expectation  $\mathbb{E}_{(\alpha_{1:T}^*, \gamma)|\beta^{(k)}, \theta^{(k)}, \Phi^{(k)}, \Sigma^{(k)}, Q^{(k)}}$ .

### • M-step

We first denote

$$\begin{aligned} \mathbf{a}_{t|T}^{*(k+1)} &= \mathbb{E}_{\alpha_{1:T}^*|\cdot}(\alpha_t^* | Y_{1:T}^*, X_{1:T}^*, \beta^{(k)}, \theta^{(k)}, \Phi^{(k)}, \Sigma^{(k)}, Q^{(k)}), \\ \mathbf{V}_{t|T}^{*(k+1)} &= \mathbb{E}_{\alpha_{1:T}^*|\cdot}(\alpha_t^* \alpha_t^{*'} | Y_{1:T}^*, X_{1:T}^*, \beta^{(k)}, \theta^{(k)}, \Phi^{(k)}, \Sigma^{(k)}, Q^{(k)}), \\ \mathbf{V}_{t,t-1|T}^{*(k+1)} &= \mathbb{E}_{\alpha_{1:T}^*|\cdot}(\alpha_t^* \alpha_{t-1}^{*'} | Y_{1:T}^*, X_{1:T}^*, \beta^{(k)}, \theta^{(k)}, \Phi^{(k)}, \Sigma^{(k)}, Q^{(k)}), \\ \mathbf{P}_{t,t-1|T}^{*(k+1)} &= \mathbf{V}_{t,t-1|T}^{*(k+1)} - \mathbf{a}_{t|T}^{*(k+1)} (\mathbf{a}_{t-1|T}^{*(k+1)})', \\ \mathbf{P}_{t|T}^{*(k+1)} &= \mathbf{V}_{t|T}^{*(k+1)} - \mathbf{a}_{t|T}^{*(k+1)} (\mathbf{a}_{t|T}^{*(k+1)})', \end{aligned}$$

and obtain  $\mathbf{a}_{t|T}^{*(k+1)}$ ,  $\mathbf{P}_{t|T}^{*(k+1)}$  and  $\mathbf{P}_{t,t-1|T}^{*(k+1)}$  from the KFBS algorithm for each  $t = 1, \dots, T$ .

We define  $\mathbf{A}_\gamma^{*(k)} = \text{diag}(a_1^{*(k)}, \dots, a_p^{*(k)})$ , recall  $a_i$  is the  $i$ -th diagonal element in  $\mathbf{A}_\gamma$ . For each  $a_i^{*(k)}$ , we have

$$a_i^{*(k)} = \mathbb{E}_{\gamma|\cdot} \left[ \frac{1}{a_i} \right] = \mathbb{E}_{\gamma|\cdot} \left[ \frac{1}{v_0(1-\gamma_i) + v_1\gamma_i} \right] = \frac{1-w_i^{(k)}}{v_0} + \frac{w_i^{(k)}}{v_1},$$

where  $w_i^{(k)} = \mathbb{E}_{\gamma|\cdot}(\gamma_i) = P(\gamma_i = 1 | \beta^{(k)}, \theta^{(k)}) = \frac{g_{1i}^{(k)}}{g_{1i}^{(k)} + g_{2i}^{(k)}}$  with

$$\begin{aligned} g_{1i}^{(k)} &= \pi(\beta_i^{(k)} | v_0, v_1, \gamma_i = 1) \theta^{(k)}, \\ g_{2i}^{(k)} &= \pi(\beta_i^{(k)} | v_0, v_1, \gamma_i = 0) (1 - \theta^{(k)}). \end{aligned}$$

Then in the  $k$ -th M-step, we maximize (2.1) with respect to  $\theta$ ,  $\beta$ ,  $\Phi$ ,  $\Sigma^{-1}$  and  $\mathbf{Q}$ . Their optimized values can be obtained by executing the following steps:

$$\begin{aligned} \theta^{(k+1)} &= \frac{\sum_{i=1}^p w_i^{(k)} + \zeta_1 - 1}{p + \zeta_1 + \zeta_2 - 2}, \\ \beta^{(k+1)} &= \left( \sum_{t=1}^T \mathbf{X}_t^{*'} (\Sigma^{(k)})^{-1} \mathbf{X}_t^* + \mathbf{A}_\gamma^{*(k+1)} \right)^{-1} \left( \sum_{t=1}^T \mathbf{X}_t^{*'} (\Sigma^{(k)})^{-1} (\mathbf{Y}_t^* - \mathbf{z} \mathbf{a}_{t|T}^{*(k+1)}) \right), \\ \text{vec}(\Phi^{(k+1)}) &= \left( \sum_{t=1}^{T-1} \left( (\mathbf{V}(\tau)_{t|T}^{*(k+1)})' \otimes (\Sigma_v^{(k)})^{-1} \right) + 10 \mathbf{I}_{n^2} \right)^{-1} \\ &\quad \times \left( \sum_{t=1}^{T-1} \left( (\mathbf{V}(\tau)_{t,t-1|T}^{*(k+1)})' \otimes (\Sigma_v^{(k)})^{-1} \right) \text{vec}(\mathbf{I}_n) \right), \\ \Sigma^{(k+1)} &= \frac{1}{T + \nu - 2} \left[ \sum_{t=1}^T (\mathbf{Y}_t^* - \mathbf{X}_t^* \beta^{(k+1)}) (\mathbf{Y}_t^* - \mathbf{X}_t^* \beta^{(k+1)})' \right. \\ &\quad - \sum_{t=1}^T \mathbf{z} \mathbf{a}_{t|T}^{*(k+1)} (\mathbf{Y}_t^* - \mathbf{X}_t^* \beta^{(k+1)})' - \sum_{t=1}^T (\mathbf{Y}_t^* - \mathbf{X}_t^* \beta^{(k+1)}) (\mathbf{a}_{t|T}^{*(k+1)})' \mathbf{z}' \\ &\quad \left. + \sum_{t=1}^T \mathbf{z} \mathbf{V}_{t|T}^{*(k+1)} \mathbf{z}' + \mathbf{H} \right] \mathbb{1}_{\{\Sigma^{-1} \in M^+(\mathcal{G})\}}, \\ \mathbf{Q}^{(k+1)} &= \frac{1}{T + \nu - 3} \left[ \left( \sum_{t=1}^{T-1} \left( \mathbf{R}' \mathbf{V}_{t+1|T}^{*(k+1)} - \mathbf{T}^{(k+1)} \mathbf{V}_{t,t+1|T}^{*(k+1)} - (\mathbf{V}_{t,t+1|T}^{*(k+1)})' (\mathbf{T}^{(k+1)})' \right. \right. \right. \\ &\quad \left. \left. + \mathbf{T}^{(k+1)} \mathbf{V}_{t|T}^{*(k+1)} (\mathbf{T}^{(k+1)})' \right) \mathbf{R} \right) \circ \begin{pmatrix} \mathbf{1}_n \mathbf{1}_n' & \mathbf{0} & \mathbf{0} \\ \mathbf{0} & \mathbf{1}_n \mathbf{1}_n' & \mathbf{0} \\ \mathbf{0} & \mathbf{0} & \mathbf{1}_n \mathbf{1}_n' \end{pmatrix} \\ &\quad \left. + \begin{pmatrix} k_1^2(n+1)\mathbf{H} & \mathbf{0} & \mathbf{0} \\ \mathbf{0} & k_2^2(n+1)\mathbf{H} & \mathbf{0} \\ \mathbf{0} & \mathbf{0} & k_3^2(n+1)\mathbf{H} \end{pmatrix} \right] \mathbb{1}_{\{\Sigma_u^{-1}, \Sigma_v^{-1}, \Sigma_w^{-1} \in M^+(\mathcal{G})\}}, \end{aligned} \tag{2.2}$$

where  $\mathbb{1}_A$  stands for the indicator function of a set  $A$ ,  $\mathbf{1}_n$  is an  $n \times 1$  vector with its elements are all 1s,  $E \circ F$  is the Hadamard product between matrices  $E$  and  $F$ ,  $\mathbf{V}(\boldsymbol{\tau})_{t|T}^{*(k+1)}$  is the covariance matrix for  $\boldsymbol{\tau}_t$  which is inside of  $\mathbf{V}_{t|T}^{*(k+1)}$ . The similar notation is used for  $\mathbf{V}(\boldsymbol{\tau})_{t,t-1|T}^{*(k+1)}$ . The E- and M-steps are repeated until the values of  $\mathcal{Q}(\boldsymbol{\beta}, \theta, \boldsymbol{\Phi}, \boldsymbol{\Sigma}, \mathbf{Q} \mid \boldsymbol{\beta}^{(k)}, \theta^{(k)}, \boldsymbol{\Phi}^{(k)}, \boldsymbol{\Sigma}^{(k)}, \mathbf{Q}^{(k)})$  stop increasing significantly. Since  $p > n$ , we can apply the Sherman-Morrison-Woodbury formula to rewrite  $(\mathbf{X}_t^{*'}(\boldsymbol{\Sigma}^{(k)})^{-1}\mathbf{X}_t^* + \mathbf{A}_\gamma^{*(k+1)})^{-1}$  in  $\boldsymbol{\beta}^{(k+1)}$  as

$$(\mathbf{A}_\gamma^{*(k+1)})^{-1} - (\mathbf{A}_\gamma^{*(k+1)})^{-1}\mathbf{X}_t^{*'}[\boldsymbol{\Sigma}^{(k)} + \mathbf{X}_t^*(\mathbf{A}_\gamma^{*(k+1)})^{-1}\mathbf{X}_t^{*'}]^{-1}\mathbf{X}_t^*(\mathbf{A}_\gamma^{*(k+1)})^{-1},$$

to only invert an  $n \times n$  matrix instead of a  $p \times p$  matrix.

### 3 Results of the new method to infer causality using the univariate model

In this section, we provide the results of the new method to infer causality by using the univariate model. Five simulated datasets are fitted into the model independently, the one-sided KS distances and their corresponding thresholds are shown in Figure 1 and Table 2.

Table 2: Results of the one-sided KS distances and thresholds obtained by applying the new method to detect causal impacts in Dataset 1, ..., Dataset 5 using the univariate model. We only present the results at the dates March 22, 2016, March 31, 2016 and April. 9, 2016 which correspond to the 1st day, 10th day and 20th day during the causal period.

|                         |             | Dataset 1 | Dataset 2 | Dataset 3 | Dataset 4 | Dataset 5 |
|-------------------------|-------------|-----------|-----------|-----------|-----------|-----------|
| March, 22<br>(1st day)  | KS distance | 0.025     | 0.024     | 0.125     | 0.107     | 0.181     |
|                         | Threshold   | 0.181     | 0.137     | 0.130     | 0.137     | 0.146     |
| March, 31<br>(10th day) | KS distance | 0.006     | 0.676     | 0.792     | 0.943     | 0.999     |
|                         | Threshold   | 0.825     | 0.618     | 0.537     | 0.501     | 0.680     |
| April, 9<br>(20th day)  | KS distance | 0.347     | 0.966     | 0.998     | 1.000     | 1.000     |
|                         | Threshold   | 0.943     | 0.851     | 0.731     | 0.780     | 0.840     |

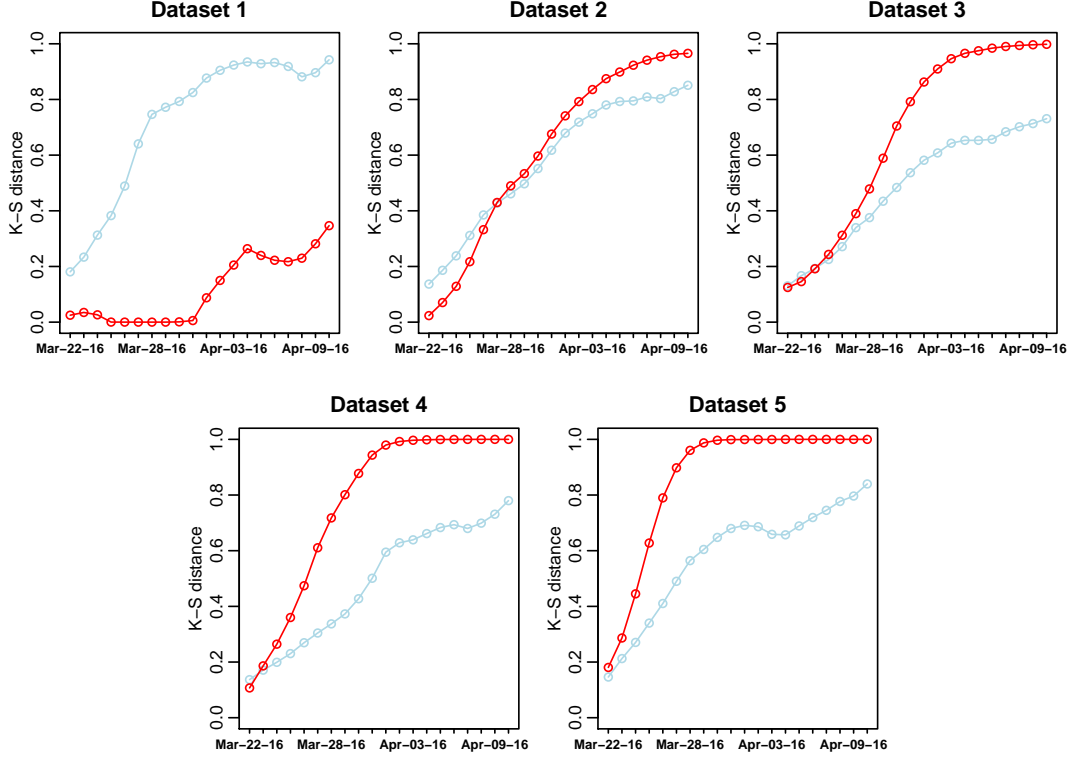

Figure 1: Results of applying the new method for detecting causal impacts in Dataset 1, ..., Dataset 5 using the univariate model during the causal period from March, 22, 2016 to April, 9, 2016. In each subplot, the red line gives the one-sided KS distances between two posterior distributions with one is given the observed data and the other is given the data of counterfactuals; the light blue line gives the corresponding thresholds.

## 4 Model checking

In this section, we present the convergence diagnostic results for MCMC chains. We also present the results for a sensitivity analysis. Furthermore, we discuss the choice of the threshold for declaring a significant impact.

### Convergence diagnostic

We conduct an MCMC convergence diagnostic based on the simulated datasets we used above. Figure 2 gives the trace plots for several parameters including the trend for Dataset 1 at time  $t = 1$ ,  $\mu_{1,1}$ ; the (1,1) coordinate element for covariance matrix  $\Sigma$ ,  $\Sigma_u$ ,  $\Sigma_v$ ,  $\Sigma_w$  and stationarity constraint matrix  $\Phi$ . From Figure 2, we see that all the six chains mix well. For each chain, the burn-in periods are short and the chain remains

stable after the burn-in period. Due the limitation of space, we do not show the trace plots for all the parameters of  $\mu_{1:T}, \tau_{1:T}, \delta_{1:T}, \Sigma, \Sigma_u, \Sigma_v, \Sigma_w$  and  $\Phi$ , but all of them have well-mixed chains.

We then use inefficient factors (IFs) to calculate the efficient draws for each MCMC chain. The formula is given as  $1 + 2 \sum_{i=1}^M (1 - i/M) \rho_i$  (see Chib, 2001), where  $\rho_i$  is the estimated autocorrelation at lag  $i$ ,  $M$  is the batch size which we take as 5000 in this simulation study. When we say that the inefficient factor has value  $M$ , this means that the number of effective draws is the total number of iterations without burn-in divided by  $M$ . Figure 3 plots the IFs for parameters in the model including all the parameters in the trend  $\mu_{1:T}$ , the covariance matrices  $\Sigma, \Sigma_u, \Sigma_v, \Sigma_w$ , the intercept for the local linear trend  $D$  and the parameters in the stationarity constraint matrix  $\Phi$ . From the plots, we observe that all the IFs except for a few parameters in  $\Phi$  are very small which suggests that the correlations are low. The large inefficient factors for parameters in  $\Phi$  occur because the use of Metropolis-Hasting algorithm, which is expected to have a larger inefficient draws than using a Gibbs sampling algorithm.

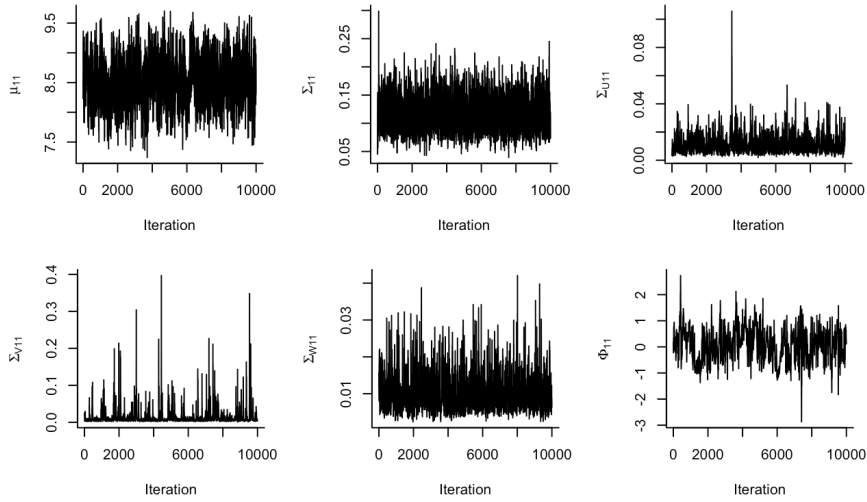

Figure 2: Traceplots for  $\mu_{11}, \Sigma_{11}, \Sigma_{u11}, \Sigma_{v11}, \Sigma_{w11}, \Phi_{11}$ .

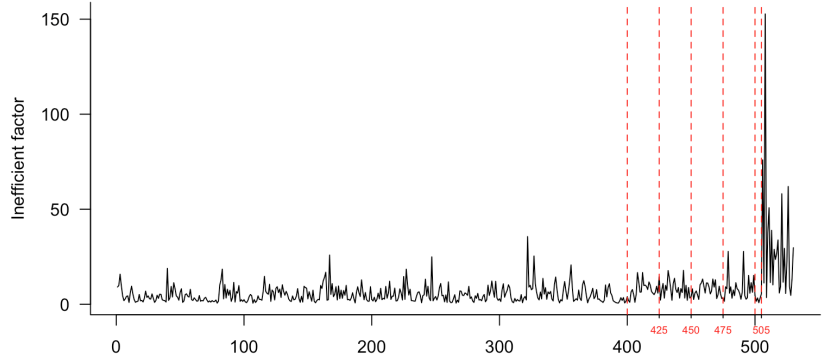

Figure 3: Plot of the inefficient factors (IFs) for  $\mu_{1:T}$ ,  $\Sigma$ ,  $\Sigma_u$ ,  $\Sigma_v$ ,  $\Sigma_w$ ,  $D$ ,  $\Phi$ . The first 400 values are IFs for parameters in  $\mu_{1:T}$  (5 datasets each with 80 time periods), the following 100 values are IFs for parameters in  $\Sigma$ ,  $\Sigma_u$ ,  $\Sigma_v$ , and  $\Sigma_w$ , with each has 25 parameters, the next 5 values are IFs for parameters in  $D$ ; and the last 25 values are IFs for parameters in  $\Phi$ . The red lines separate IFs result from different parameters.

### Sensitivity analysis

Consider the following model,

$$\begin{aligned} Y_t &= z\alpha_t + X_t\beta + \varrho_t\epsilon_t, \\ \alpha_{t+1} &= c + T\alpha_t + R\eta_t. \end{aligned} \quad (4.1)$$

where  $\varrho_t$ s are random draws from an exponential distribution with mean equal to 1. Thus the error is heteroskedastic with a heavy tail. We generate the data from (4.1) but use the model (3.1) of our paper to conduct the causal inference. The data generating process is similar to the one described in our paper. We apply both the commonly used method and the new method to estimate the causal effects of the simulated datasets. The results for using the commonly used method are shown in Table 3 and the results for using the new method are shown in Table 4 and Figure 4.

From Table 3, the commonly used method fails to detect the causal impact for Dataset 2 and 4. Even though Dataset 4 has a relatively large impact. However, from

Table 3: Posterior medians and 95% credible intervals of average causal impacts for the model (4.1).

|           | Simulated impact | Posterior median | 95% credible intervals |
|-----------|------------------|------------------|------------------------|
| Dataset 1 | 0.00             | -0.03            | [-2.177, 2.233]        |
| Dataset 2 | 1.06             | 1.81             | [-0.421, 4.044]        |
| Dataset 3 | 2.12             | 2.65             | [0.520, 5.193]         |
| Dataset 4 | 3.18             | 2.71             | [-0.393, 5.102]        |
| Dataset 5 | 4.23             | 4.28             | [2.108, 6.000]         |

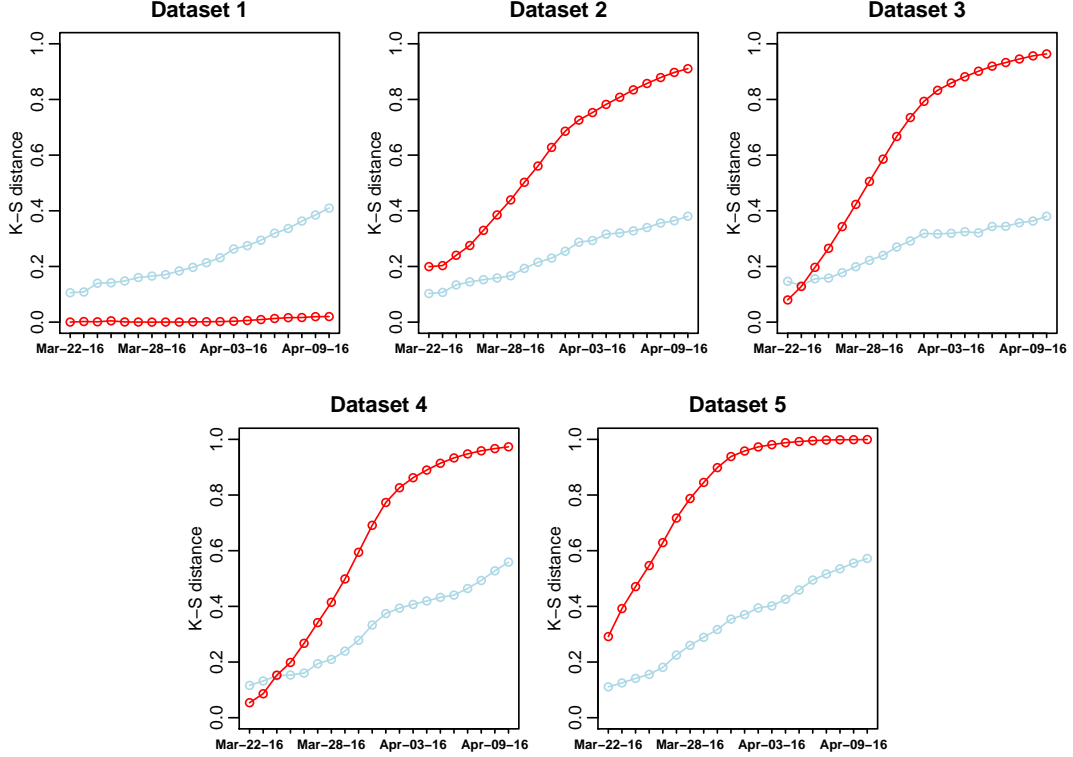

Figure 4: Results of applying the new method for detecting causal impacts in Dataset 1, ..., Dataset 5 with the data generated from model (4.1) during the causal period from March, 22, 2016 to April, 9, 2016. In each subplot, the red line gives the one-sided KS distances between two posterior distributions with one is given the observed data and the other given the data of counterfactuals; the light blue line gives the corresponding thresholds.

Table 4 and Figure 4, we found that by using the new method, all the Datasets containing causal impact are successfully detected. Our method also does a good job on distinguishing the datasets containing causal impacts with the one not containing any causal impacts.

Table 4: Results of the one-sided KS distances and thresholds obtained by applying the new method to detect causal impacts in Dataset 1, . . . , Dataset 5 using the model (4.1) with the stationarity constraint. We only present the results at the dates March 22, 2016, March 31, 2016 and April. 9, 2016 which correspond to the 1st day, 10th day and 20th day during the causal period.

|                         |             | Dataset 1 | Dataset 2 | Dataset 3 | Dataset 4 | Dataset 5 |
|-------------------------|-------------|-----------|-----------|-----------|-----------|-----------|
| March, 22<br>(1st day)  | KS distance | 0.000     | 0.199     | 0.080     | 0.054     | 0.292     |
|                         | Threshold   | 0.106     | 0.103     | 0.147     | 0.116     | 0.111     |
| March, 31<br>(10th day) | KS distance | 0.001     | 0.628     | 0.735     | 0.691     | 0.938     |
|                         | Threshold   | 0.197     | 0.230     | 0.292     | 0.333     | 0.354     |
| April, 9<br>(20th day)  | KS distance | 0.020     | 0.911     | 0.964     | 0.973     | 0.999     |
|                         | Threshold   | 0.410     | 0.380     | 0.380     | 0.559     | 0.572     |

### Using a threshold by choosing a different percentile

In our paper, we proposed using the 95% upper percentile to calculate the threshold for detecting a significant impact. If we choose a higher percentile, it becomes more difficult to detect an impact. On the other hand, it prevents false discoveries. We then conduct a study by using the 99% upper percentile for the same simulated datasets. We plot the results in Figure 5. Compared with Figure 5 of our paper, the thresholds in Figure 5 are randomly larger for all the subplots. However, we can still successfully detect the causal impacts in all the datasets.

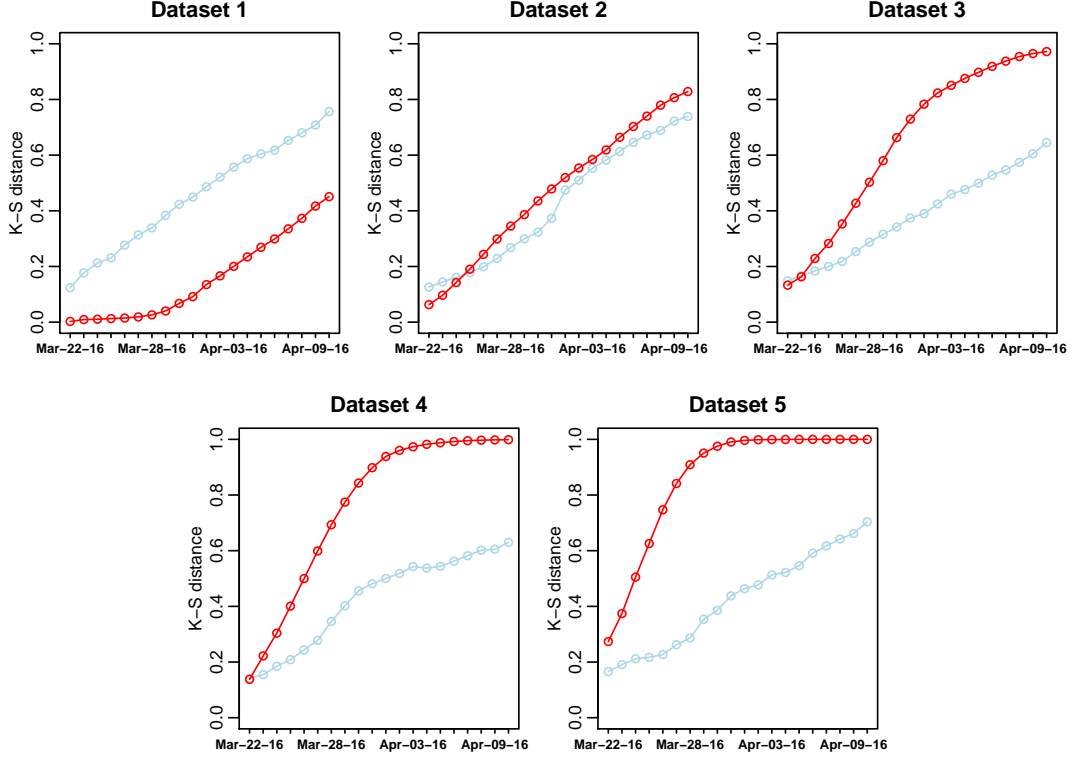

Figure 5: Results of applying the new method for detecting causal impacts in Dataset 1, ..., Dataset 5 during the causal period from March, 22, 2016 to April, 9, 2016 with thresholds chosen as the 99% upper percentile from the one-sided KS distances obtained from 30 generated counterfactuals. In each subplot, the red line gives the one-sided KS distances between two posterior distributions with one is given the observed data and the other is given their corresponding counterfactuals; the light blue line gives the corresponding thresholds.

## 5 The Kalman filter and backward smoothing algorithm

For the following state-space model

$$\begin{aligned} Y_t &= z\alpha_t + X_t\beta + \epsilon_t, \\ \alpha_{t+1} &= c + T\alpha_t + R\eta_t, \end{aligned}$$

where  $\epsilon_t \sim \mathcal{N}(\mathbf{0}, \Sigma)$ ,  $\eta \sim \mathcal{N}(\mathbf{0}, Q)$ ,  $Q = \text{bdiag}(\Sigma_u, \Sigma_v, \Sigma_w)$  are mutually independent, the [Durbin and Koopman \(2002\)](#)'s KFBS algorithm is described as follows: for a dataset with no missing values, the Kalman filter for updating  $\alpha_t$ , where  $\alpha_t \sim \mathcal{N}(a_t, P_t)$ ,

$t = 1, \dots, T$ , is given by

$$\begin{aligned} \mathbf{v}_t &= \mathbf{Y}_t - \mathbf{z}\mathbf{a}_t, & \mathbf{F}_t &= \mathbf{z}\mathbf{P}_t\mathbf{z}' + \Sigma, \\ \mathbf{K}_t &= \mathbf{T}\mathbf{P}_t\mathbf{z}'\mathbf{F}_t^{-1}, & \mathbf{L}_t &= \mathbf{T} - \mathbf{K}_t\mathbf{z}, \\ \mathbf{a}_{t+1} &= \mathbf{c} + \mathbf{T}\mathbf{a}_t + \mathbf{K}_t\mathbf{v}_t, & \mathbf{P}_{t+1} &= \mathbf{T}\mathbf{P}_t\mathbf{L}_t' + \mathbf{R}\mathbf{Q}\mathbf{R}'. \end{aligned}$$

For updating the missing values in the dataset, the Kalman filter algorithm becomes

$$\mathbf{a}_{t+1} = \mathbf{c} + \mathbf{T}\mathbf{a}_t, \quad \mathbf{P}_{t+1} = \mathbf{T}\mathbf{P}_t\mathbf{T}' + \mathbf{R}\mathbf{Q}\mathbf{R}'.$$

From the above, we obtain  $\mathbf{a}_{t+1}$  and  $\mathbf{P}_{t+1}$  depending on the data  $\mathbf{Y}_1, \dots, \mathbf{Y}_t$ . The backward smoothing algorithm will give the conditional expectation of  $\mathbf{a}_t$  and  $\mathbf{P}_t$  given the full dataset  $\mathbf{Y}_1, \dots, \mathbf{Y}_T$ . To distinguish between those two values, we denote the latter one as  $\mathbf{a}_{t|T}$  and  $\mathbf{P}_{t|T}$ .

The backward smoothing algorithm is given by

$$\begin{aligned} \mathbf{r}_{t-1} &= \mathbf{z}'\mathbf{F}_t^{-1}\mathbf{v}_t + \mathbf{L}_t'\mathbf{r}_t, & \mathbf{N}_{t-1} &= \mathbf{z}'\mathbf{F}_t^{-1}\mathbf{z} + \mathbf{L}_t'\mathbf{N}_t\mathbf{L}_t, \\ \mathbf{a}_{t|T} &= \mathbf{a}_t + \mathbf{P}_t\mathbf{r}_{t-1}, & \mathbf{P}_{t|T} &= \mathbf{P}_t - \mathbf{P}_t\mathbf{N}_{t-1}\mathbf{P}_t. \end{aligned}$$

The covariance between  $\alpha_t$  and  $\alpha_{t-1}$  is given by

$$\mathbf{P}_{t-1,t|T} = \text{cov}(\alpha_{t-1}, \alpha_t | \mathbf{Y}_1, \dots, \mathbf{Y}_T) = \mathbf{P}_{t-1}\mathbf{L}_{t-1}'(\mathbf{I} - \mathbf{N}_{t-1}\mathbf{P}_t).$$

## References

- Chib, S. (2001). *Markov Chain Monte Carlo Methods: Computation and Inference in Handbook of Econometrics, vol. 5*. North-Holland, Amsterdam: Elsevier. [9](#)
- Dawid, A. P. and S. L. Lauritzen (1993). Hyper-Markov laws in the statistical analysis of decomposable graphical models. *The Annals of Statistics* *21*, 1272–1317. [4](#)
- Durbin, J. and S. J. Koopman (2002). A simple and efficient simulation smoother for state space time series analysis. *Biometrika* *89*, 603–615. [3](#), [13](#)
- Durbin, J. and S. J. Koopman (2012). *Time Series Analysis by State Space Methods: Second Edition*. Great Clarendon Street, Oxford OX2 6DP: Oxford University Press. [3](#)
- Mohammadi, A. and E. C. Wit (2015). Bayesian structure learning in sparse Gaussian graphical models. *Bayesian Analysis* *10*, 109–138. [4](#)
- Primiceri, G. E. (2005). Time varying structural vector autoregressions and monetary policy. *The Review of Economic Studies* *72*, 821–852. [3](#)
- Roverato, A. (2000). Cholesky decomposition of a hyper inverse Wishart matrix. *Biometrika* *87*, 99–112. [4](#)
- Roverato, A. (2002). Hyper inverse Wishart distribution for non-decomposable graphs and its application to Bayesian inference for Gaussian graphical models. *Scandinavian Journal of Statistics* *29*, 391–411. [4](#)

Shephard, N. and M. K. Pitt (1997). Likelihood analysis of non-Gaussian measurement time series. *Biometrika* 84, 653–667. [3](#)
