# Supplementary material for: Bayesian method for causal inference in spatially-correlated multivariate time series
Source: arXiv:1801.06282 source file (2018-03-12)
Supplement: Supplementary file 2 [file appendix-A.tex]

\section{The Kalman filter and backward smoothing algorithm}
\label{app-A}

We consider the state-space model described in (\ref{equ-2.6}) and (\ref{equ-2.7}).
The \citet{durb02}'s KFBS algorithm is described as follows:
for a dataset with no missing values, the Kalman filter for updating 
$\boldsymbol \alpha_t$,
where $\boldsymbol \alpha_t \sim \mathcal{N}(\boldsymbol a_t, \boldsymbol P_t)$, 
$t = 1, \dots, T$, is given by
\begin{equation*}
\begin{split}
     \boldsymbol v_t 
     = 
     \boldsymbol Y_t - \boldsymbol z \boldsymbol a_t, \quad
     &\boldsymbol F_t  
     = 
     \boldsymbol z \boldsymbol P_t \boldsymbol z' + 
     \boldsymbol \Sigma,\\
     \boldsymbol K_t  
      =  
     \boldsymbol T \boldsymbol P_t \boldsymbol z'
     \boldsymbol F_t^{-1},
     \quad
     &\boldsymbol L_t
     =
     \boldsymbol T - \boldsymbol K_t \boldsymbol z,\\
     \boldsymbol a_{t+1} 
      = \boldsymbol c 
     + \boldsymbol T \boldsymbol a_t 
     + \boldsymbol K_t \boldsymbol v_t,
     \quad       
     &\boldsymbol P_{t+1}
     = 
     \boldsymbol T \boldsymbol P_t \boldsymbol L_t'
     + 
     \boldsymbol R \boldsymbol Q \boldsymbol R'.
\end{split}
\end{equation*}
For updating the missing values in the dataset, 
the Kalman filter algorithm becomes 
\begin{eqnarray*}
      \boldsymbol a_{t+1}  = \ \boldsymbol c + 
        \boldsymbol T \boldsymbol a_t, \quad
      \boldsymbol P_{t+1} = \ \boldsymbol T \boldsymbol P_t  \boldsymbol T' +
         \boldsymbol R \boldsymbol Q \boldsymbol R'.
\end{eqnarray*}

From the above, we obtain $\boldsymbol a_{t+1}$ and $\boldsymbol P_{t+1}$ depending on the data $\boldsymbol Y_1, \dots, \boldsymbol Y_{t}$.
The backward smoothing algorithm will give the conditional expectation of $\boldsymbol a_t$ and $\boldsymbol P_t$ given the full dataset $\boldsymbol Y_1, \dots, \boldsymbol Y_T$. 
To distinguish between those two values, we denote the latter one as $\boldsymbol a_{t|T}$ and $\boldsymbol P_{t|T}$.

The backward smoothing algorithm is given by
\begin{equation*}
\begin{split}
    \boldsymbol r_{t-1} 
     = 
    \boldsymbol z'
    \boldsymbol F_t^{-1}
    \boldsymbol v_t
    +
    \boldsymbol L_t'
    \boldsymbol r_t,
    \quad
    &\boldsymbol N_{t-1}
    =
    \boldsymbol z'
    \boldsymbol F_t^{-1}
    \boldsymbol z
    +
    \boldsymbol L_t'
    \boldsymbol N_t
    \boldsymbol L_t,\\
    \boldsymbol a_{t|T}
     = 
    \boldsymbol a_{t} +
    \boldsymbol P_t
    \boldsymbol r_{t-1}, 
    \quad 
    &\boldsymbol P_{t|T}
    =
    \boldsymbol P_t
    -
    \boldsymbol P_t
    \boldsymbol N_{t-1}
    \boldsymbol P_t.
\end{split}
\end{equation*}

The covariance between $\boldsymbol\alpha_t$ and $\boldsymbol\alpha_{t-1}$ is given by
\begin{equation*}
    \boldsymbol P_{t-1, t|T}
    =
\text{cov}(\boldsymbol \alpha_{t-1}, \boldsymbol \alpha_{t}| 
\boldsymbol Y_1, \dots, \boldsymbol Y_T)
    =
    \boldsymbol P_{t-1} \boldsymbol L_{t-1}'
    (\boldsymbol I
    -
    \boldsymbol N_{t-1} \boldsymbol P_{t}).
\end{equation*}
