# Supplementary material for: Bayesian method for causal inference in spatially-correlated multivariate time series
Source: arXiv:1801.06282 source file (2018-03-12)
Supplement: Supplementary file 3 [file appendix-B.tex]

\section{Details on deriving EMVS}
\label{app-B}

This section gives the details of the derivation of the EMVS algorithm in
Section \ref{sec-3.1}.
From (\ref{equ-3.1})--(\ref{equ-3.3}) we have, with a constant $C$,
\begin{equation*}
\begin{split}
    \mathcal{Q}( &\boldsymbol \beta, \theta, \boldsymbol \Phi, 
    \boldsymbol \Sigma, \boldsymbol Q
        \ | \ \boldsymbol \beta^{(k)}, \theta^{(k)}, \boldsymbol \Phi^{(k)}, \boldsymbol \Sigma^{(k)}, \boldsymbol Q^{(k)}
    ) \\
    & = C +  \mathcal{Q}_1( \boldsymbol \beta, \boldsymbol \Phi, 
    \boldsymbol \Sigma, \boldsymbol Q
          \ | \ \boldsymbol \beta^{(k)}, \theta^{(k)}, \boldsymbol \Phi^{(k)}, \boldsymbol \Sigma^{(k)}, \boldsymbol Q^{(k)}
         )
     + \mathcal{Q}_2(\theta
          \ | \ \boldsymbol \beta^{(k)}, \theta^{(k)}
         ),
\end{split}
\end{equation*}
where
\begin{align*}
     \mathcal{Q}_1( &\boldsymbol \beta, \boldsymbol \Phi, 
    \boldsymbol \Sigma, \boldsymbol Q
          \ | \ \boldsymbol \beta^{(k)}, \theta^{(k)}, \boldsymbol \Phi^{(k)}, \boldsymbol \Sigma^{(k)}, \boldsymbol Q^{(k)}
         )\\
     & = 
     - \frac{1}{2} \sum_{t=1}^T  
     	\mathbb{E}_{\boldsymbol \alpha_{1:T}^*|\cdot}
     	\Big[
     	(\boldsymbol Y_t^* 
     	- \boldsymbol X_t^* \boldsymbol \beta
     	- \boldsymbol z \boldsymbol \alpha_t^*)'
        \boldsymbol \Sigma^{-1}
       (\boldsymbol Y_t^*
       - \boldsymbol X_t^* \boldsymbol \beta
       - \boldsymbol z \boldsymbol \alpha_t^*)
       \Big]\\ 
    & \quad
    - \frac{1}{2} \sum_{t=1}^{T-1}
    \mathbb{E}_{\boldsymbol \alpha_{1:T}^*|\cdot}
    \Big[
        (\boldsymbol \alpha_{t+1}^* 
        - \boldsymbol T \boldsymbol \alpha_t^*)' 
        \boldsymbol R \boldsymbol Q^{-1} \boldsymbol R'
        (\boldsymbol \alpha_{t+1}^* 
        - \boldsymbol T \boldsymbol \alpha_t^*)
    \Big]
    - \frac{1}{2} 
    {\boldsymbol \alpha_1^*}' \boldsymbol \alpha_1^*\\
     & \quad 
     + \frac{T+\nu-2}{2} \log |\boldsymbol \Sigma^{-1}| 
     + \frac{T+\nu-3}{2} 
     \Big(\log|\boldsymbol \Sigma_u^{-1}|
     + \log |\boldsymbol \Sigma_v^{-1}| 
     + \log |\boldsymbol \Sigma_w^{-1}|
     \Big)\\
     & \quad 
    - \frac{1}{2} \Big(\Tr(\boldsymbol H \boldsymbol \Sigma^{-1})
    + \Tr(k_1^2(n+1) \boldsymbol H \boldsymbol \Sigma_u^{-1})
    + \Tr(k_2^2(n+1) \boldsymbol H \boldsymbol \Sigma_v^{-1})
    + \Tr(k_3^2(n+1) \boldsymbol H \boldsymbol \Sigma_w^{-1}) 
    \Big)\\
    & \quad
    - \frac{1}{2 \times 0.1} \text{vec}(\boldsymbol \Phi)' \text{vec}(\boldsymbol \Phi)
    - \sum_{i=1}^p \mathbb{E}_{\boldsymbol \gamma| \cdot}\big[ \log\big(v_0(1-\gamma_i) + v_1 \gamma_i\big) \big] \\
    & \quad 
    - \frac{1}{2} \sum_{i=1}^{p} \beta_i^2 \ \mathbb{E}_{\boldsymbol \gamma| \cdot}
             \Big[\frac{1}{v_0 (1-\gamma_i) + v_1 \gamma_i} \Big],
\end{align*}
and 
\begin{equation*}
\begin{split}
     &\mathcal{Q}_2( \theta
          \ | \ \boldsymbol \beta^{(k)}, \theta^{(k)}
        )\\
     & \quad = 
     \sum_{i=1}^p \log \Big ( \frac{\theta}{1-\theta} \Big) 
     \mathbb{E}_{\boldsymbol \gamma| \cdot} (\gamma_i)
     + (\zeta_1 - 1) \log \theta + (p + \zeta_2 -1) \log (1-\theta).
\end{split}  
\end{equation*}

The expectation of 
$\boldsymbol \alpha_t^*$, 
$\boldsymbol \alpha_t^* {\boldsymbol \alpha_t^*}'$
and 
$\boldsymbol \alpha_t^* {\boldsymbol \alpha_{t-1}^*}'$
respect to $\boldsymbol \alpha_{1:T}^*|\cdot$
can be estimated using the KFBS algorithm (see details in Appendix \ref{app-A}).

The term 
$\mathbb{E}_{\boldsymbol \gamma| \cdot}\big[
\log \big(v_0(1-\gamma_i) + v_1 \gamma_i\big) \big]$
is a constant when conditioned on the parameters 
$\boldsymbol \beta^{(k)}, v_0, v_1$.

Let
$
a_i^{*(k)} = \mathbb{E}_{\boldsymbol \gamma| \cdot} 
                \Big[\frac{1}{v_0 (1-\gamma_i) + v_1 \gamma_i} \Big]
$,
because $\gamma_i$ is a binary variable, we have
\begin{equation*}
\begin{split}
   a_i^{*(k)} = \mathbb{E}_{\boldsymbol \gamma| \cdot} 
                \Big[\frac{1}{v_0 (1-\gamma_i) + v_1 \gamma_i} \Big]
   =
   \frac{\mathbb{E}_{\boldsymbol \gamma| \cdot} (1-\gamma_i)}{v_0} + 
   \frac{\mathbb{E}_{\boldsymbol \gamma| \cdot} (\gamma_i)}{v_1}.
\end{split}   
\end{equation*}

We let 
$w_i^{(k)} = \mathbb{E}_{\boldsymbol \gamma| \cdot} (\gamma_i)$,
then
\begin{equation*}
w_i^{(k)} = 
\mathbb{E}_{\boldsymbol \gamma| \cdot} (\gamma_i)
=
P(\gamma_i = 1 \ | \
\boldsymbol \beta^{(k)}, \theta^{(k)} ) 
=\frac{g_{1i}^{(k)}}{g_{1i}^{(k)} + g_{2i}^{(k)}},
\end{equation*}
where 
$g_{1i}^{(k)} = \pi(\beta_i^{(k)}| v_0, v_1, \gamma_i = 1)
P(\gamma_i = 1 | \theta^{(k)})$ and 
$g_{2i}^{(k)} = \pi(\beta_i^{(k)}| v_0, v_1, \gamma_i = 0)
P(\gamma_i = 0 | \theta^{(k)})$.
Furthermore, based on the prior in Section \ref{sec-2}, 
$g_{1i}^{(k)}$ and $g_{2i}^{(k)}$ can be written as 
$g_{1i}^{(k)} = \pi(\beta_i^{(k)}| v_0, v_1, \gamma_i = 1)\theta^{(k)}$ 
and 
$g_{2i}^{(k)} = \pi(\beta_i^{(k)}| v_0, v_1, \gamma_i = 0)
(1-\theta^{(k)})$.

If using DAEMVS algorithm with parameter $s$, then 
\begin{align*}
w_i^{(k)} = \frac{\big(g_{1i}^{(k)}\big)^s}
{\big(g_{1i}^{(k)}\big)^s + \big(g_{2i}^{(k)}\big)^s}.
\end{align*}

In the M-step, we plug-in these expression in (\ref{equ-3.3}). After taking derivative respects
to $\theta$, $\boldsymbol \beta$, $\boldsymbol \Phi$, 
$\boldsymbol \Sigma$ and $\boldsymbol Q$,
we obtain the expressions in (\ref{equ-3.4}).

Here we outline the revised EMVS algorithm.
The algorithm contains two steps:
the expectation step (E-step) and the maximization step (M-step).

\begin{itemize}
    \item {\bf E-step}
\end{itemize}

In the $k$-th E-step,
we find
\begin{equation}
\label{equ-3.3}
\begin{split}
    & \mathcal{Q}( \boldsymbol \beta, \theta, \boldsymbol \Phi, 
    \boldsymbol \Sigma, \boldsymbol Q
        \ | \ \boldsymbol \beta^{(k)}, \theta^{(k)}, \boldsymbol \Phi^{(k)}, \boldsymbol \Sigma^{(k)}, \boldsymbol Q^{(k)}
    ) \\
    & = 
    \mathbb{E}_{(\boldsymbol \alpha_{1:T}^*, \boldsymbol \gamma)| \cdot} 
\big[ 
    \log \pi(\boldsymbol \alpha_{1:T}^*, \boldsymbol \beta, 
    \boldsymbol \gamma, \theta, \boldsymbol \Phi,
    \boldsymbol \Sigma, \boldsymbol Q
    | \boldsymbol Y_t^*, \boldsymbol X_t^*)\ | 
    \ \boldsymbol \beta^{(k)}, \theta^{(k)}, \boldsymbol \Phi^{(k)}, \boldsymbol \Sigma^{(k)}, \boldsymbol Q^{(k)}
\big],
\end{split}
\end{equation}
where 
 $\mathbb{E}_{(\boldsymbol \alpha_{1:T}^*, \boldsymbol \gamma)| \cdot}(\cdot)$ denotes the conditional 
expectation 
$\mathbb{E}_{(\boldsymbol \alpha_{1:T}^*, \boldsymbol \gamma)| 
\boldsymbol \beta^{(k)}, \theta^{(k)}, \boldsymbol \Phi^{(k)}, \boldsymbol \Sigma^{(k)}, \boldsymbol Q^{(k)}}$.

We denote
\begin{equation*}
\begin{split}
\boldsymbol a_{t|T}^{*(k+1)}
& =  
\mathbb{E}_{\boldsymbol \alpha_{1:T}^*|\cdot}
(\boldsymbol \alpha_t^* \ | \ 
\boldsymbol Y_{1:T}^*, \boldsymbol X_{1:T}^*,
\boldsymbol \beta^{(k)}, \theta^{(k)}, \boldsymbol \Phi^{(k)}, \boldsymbol \Sigma^{(k)}, \boldsymbol Q^{(k)}),\\
\boldsymbol V_{t|T}^{*(k+1)} 
& =  
\mathbb{E}_{\boldsymbol \alpha_{1:T}^*|\cdot}
(\boldsymbol \alpha_t^* {\boldsymbol \alpha_t^*}' \ | \
\boldsymbol Y_{1:T}^*, \boldsymbol X_{1:T}^*,
\boldsymbol \beta^{(k)}, \theta^{(k)}, \boldsymbol \Phi^{(k)}, \boldsymbol \Sigma^{(k)}, \boldsymbol Q^{(k)}),\\
\boldsymbol V_{t, t-1|T}^{*(k+1)} 
& =
\mathbb{E}_{\boldsymbol \alpha_{1:T}^*|\cdot}
(\boldsymbol \alpha_t^* {\boldsymbol \alpha_{t-1}^*}' \ |\
\boldsymbol Y_{1:T}^*, \boldsymbol X_{1:T}^*,\boldsymbol \beta^{(k)}, \theta^{(k)}, \boldsymbol \Phi^{(k)}, \boldsymbol \Sigma^{(k)}, \boldsymbol Q^{(k)}), \\
\boldsymbol P_{t, t-1|T}^{*(k+1)} 
& = 
\boldsymbol V_{t, t-1|T}^{*(k+1)} 
- \boldsymbol a_{t|T}^{*(k+1)} \big(\boldsymbol a_{t-1|T}^{*(k+1)}\big)',\\
\boldsymbol P_{t|T}^{*(k+1)} 
& = 
\boldsymbol V_{t|T}^{*(k+1)} 
- \boldsymbol a_{t|T}^{*(k+1)} 
\big(\boldsymbol a_{t|T}^{*(k+1)}\big)',
\end{split}
\end{equation*}
and obtain
$\boldsymbol a_{t|T}^{*(k+1)}$, 
$\boldsymbol P_{t|T}^{*(k+1)}$
and 
$\boldsymbol P_{t, t-1|T}^{*(k+1)}$
from the KFBS algorithm (see Appendix \ref{app-A}) for each $t = 1, \dots, T$.

We define
$\boldsymbol A_{\boldsymbol \gamma}^{*(k)}
=
(a_1^{*(k)}, \dots, a_p^{*(k)}).
$
For each $a_i^{*(k)}$, we have
\begin{align*}
    a_i^{*(k)} = \mathbb{E}_{\boldsymbol \gamma| \cdot} 
                \Big[\frac{1}{a_i} \Big]
        =\mathbb{E}_{\boldsymbol \gamma| \cdot} 
                \Big[\frac{1}{v_0 (1-\gamma_i) + v_1 \gamma_i} \Big]
            = \frac{1-w_i^{(k)}}{v_0} + \frac{w_i^{(k)}}{v_1},    
\end{align*}
where 
$w_i^{(k)} = 
\mathbb{E}_{\boldsymbol \gamma| \cdot}(\gamma_i)
= P(\gamma_i = 1| \boldsymbol \beta^{(k)}, \theta^{(k)}) =
\frac{g_{1i}^{(k)}}{g_{1i}^{(k)} + g_{2i}^{(k)}}$ with
\begin{align*}
    g_{1i}^{(k)} &= \pi(\beta_i^{(k)}| v_0, v_1, \gamma_i = 1)\theta^{(k)},\\
    g_{2i}^{(k)} &= \pi(\beta_i^{(k)}| v_0, v_1, \gamma_i = 0)(1-\theta^{(k)}).
\end{align*}
Recall $a_i$ is the $i$-th diagonal element in $\boldsymbol A_{\boldsymbol \gamma}$.

\begin{itemize}
    \item {\bf M-step}
\end{itemize}

In the $k$-th M-step, we maximize (\ref{equ-3.3}) with respect to
$\theta$,
$\boldsymbol \beta$, 
$\boldsymbol \Phi$,
$\boldsymbol \Sigma^{-1}$ and $\boldsymbol Q$.
Their optimized values can be obtained by
executing the following steps:
\begin{align}
\label{equ-3.4}
    \theta^{(k+1)} 
   & = 
   \frac{\sum_{i=1}^p w_i^{(k)} + \zeta_1 - 1}{p + \zeta_1 + \zeta_2 - 2},
   \nonumber\\
   \boldsymbol \beta^{(k+1)} 
   & =  
   \Big(
   \sum_{t=1}^T \boldsymbol X_t^{*}' (\boldsymbol \Sigma^{(k)})^{-1} \boldsymbol X_t^*
    + \boldsymbol A_{\boldsymbol \gamma}^{*(k+1)}
    \Big)^{-1}
    \Big(
    \sum_{t=1}^T
   \boldsymbol X_t^{*}' (\boldsymbol \Sigma^{(k)})^{-1} (\boldsymbol Y_t^* - \boldsymbol z \boldsymbol a_{t|T}^{*(k+1)})
   \Big),
   \nonumber\\
   \text{vec}(\boldsymbol \Phi^{(k+1)})
   & = 
   \Big(
    \sum_{t=1}^{T-1} 
    \Big(\big(\boldsymbol V(\boldsymbol \tau)_{t|T}^{*(k+1)}\big)'
    \otimes
    (\boldsymbol \Sigma_v^{(k)})^{-1}
    \Big)
    +
    10 \boldsymbol I_{n^2}
   \Big)^{-1} 
   \nonumber \\
    & \quad \times \Big(
    \sum_{t=1}^{T-1}
    \Big(
    \big(\boldsymbol V(\boldsymbol \tau)_{t, t-1|T}^{*(k+1)}\big)'
    \otimes
    (\boldsymbol \Sigma_v^{(k)})^{-1} 
    \Big)\text{vec}(\boldsymbol I_n)
   \Big),
   \nonumber\\
   \boldsymbol \Sigma^{(k+1)} 
   & = 
   \frac{1}{T+ \nu - 2}
   \big[
   \sum_{t=1}^T
   (\boldsymbol Y_t^* 
   - \boldsymbol X_t^* \boldsymbol \beta^{(k+1)})
   (\boldsymbol Y_t^* 
   - \boldsymbol X_t^* \boldsymbol \beta^{(k+1)})' 
   \nonumber\\
   & \quad 
   - \sum_{t=1}^T
   \boldsymbol z \boldsymbol a_{t|T}^{*(k+1)} 
   (\boldsymbol Y_t^* 
   - \boldsymbol X_t^* \boldsymbol \beta^{(k+1)})'
   - \sum_{t=1}^T
   (\boldsymbol Y_t^* 
   - \boldsymbol X_t^* \boldsymbol \beta^{(k+1)})
   \big(\boldsymbol a_{t|T}^{*(k+1)}\big)'
   \boldsymbol z' 
   \nonumber\\
   & \quad + \sum_{t=1}^T
   \boldsymbol z 
   \boldsymbol V_{t|T}^{*(k+1)}
   \boldsymbol z'
   + \boldsymbol H 
   \Big]
   \mathbbm{1}_{\{\boldsymbol \Sigma^{-1} \in M^+(\mathcal{G}) \}}, 
   \nonumber\\
   \boldsymbol Q^{(k+1)}
   & = \frac{1}{T + \nu - 3}
   \Big[
   \Big(
   \sum_{t=1}^{T-1}
   \Big(
    \boldsymbol R' 
        \boldsymbol V_{t+1|T}^{*(k+1)}
        - \boldsymbol T^{(k+1)} \boldsymbol V_{t, t+1|T}^{*(k+1)}
        - \big(\boldsymbol V_{t, t+1|T}^{*(k+1)}\big)'
        \big(\boldsymbol T^{(k+1)}\big)'
        \nonumber\\
        & \quad 
        + \boldsymbol T^{(k+1)} \boldsymbol V_{t|T}^{*(k+1)}
        \big(\boldsymbol T^{(k+1)}\big)'
    \Big) \boldsymbol R  \Big)
   \circ 
   \begin{pmatrix}
   \boldsymbol 1_n\boldsymbol 1_n' & \boldsymbol 0 & \boldsymbol 0\\
   \boldsymbol 0 & \boldsymbol 1_n\boldsymbol 1_n' & \boldsymbol 0\\
   \boldsymbol 0 & \boldsymbol 0 & \boldsymbol 1_n\boldsymbol 1_n'
   \end{pmatrix}
   \nonumber\\
   & \quad +
    \begin{pmatrix}
        k_1^2(n+1)\boldsymbol H & \boldsymbol 0& \boldsymbol 0\\
        \boldsymbol 0 & k_2^2(n+1)\boldsymbol H & \boldsymbol 0\\
        \boldsymbol 0 & \boldsymbol 0 & k_3^2(n+1)\boldsymbol H
    \end{pmatrix}
   \Big]
   \mathbbm{1}_{\{\boldsymbol \Sigma_u^{-1},
   \boldsymbol \Sigma_v^{-1},
   \boldsymbol \Sigma_w^{-1} \in M^+(\mathcal{G}) \}},
\end{align}
where $\mathbbm{1}_A$ stands for the indicator function of a set $A$, 
$\boldsymbol 1_n$ is an $n \times 1$ vector with its elements are all $1$s,
$E \circ F$ is the Hadamard product between matrices $E$ and $F$,
$\boldsymbol V(\boldsymbol \tau)_{t|T}^{*(k+1)}$
is the covariance matrix for $\boldsymbol \tau_t$ 
which is inside of $\boldsymbol V_{t|T}^{*(k+1)}$.
The similar notation is used for 
$\boldsymbol V(\boldsymbol \tau)_{t, t-1|T}^{*(k+1)}$.
The E- and M-steps are repeated until the values of 
$\mathcal{Q}( \boldsymbol \beta, \theta, \boldsymbol \Phi, 
    \boldsymbol \Sigma, \boldsymbol Q
        \ | \ \boldsymbol \beta^{(k)}, \theta^{(k)}, \boldsymbol \Phi^{(k)}, \boldsymbol \Sigma^{(k)}, \boldsymbol Q^{(k)}
    )$ stop increasing significantly.
Since $p > n$, 
we can apply the
Sherman-Morrison-Woodbury formula 
to rewrite
$({\boldsymbol X_t^{*}}' (\boldsymbol \Sigma^{(k)})^{-1} \boldsymbol X_t^*
+ \boldsymbol A_{\boldsymbol \gamma}^{*(k+1)})^{-1}$
in $\boldsymbol \beta^{(k+1)}$
as
\begin{equation*}
    (\boldsymbol A_{\boldsymbol \gamma}^{*(k+1)})^{-1} -
    (\boldsymbol A_{\boldsymbol \gamma}^{*(k+1)})^{-1} 
    {\boldsymbol X_t^{*}}'  
    [
    \boldsymbol \Sigma^{(k)} + 
    \boldsymbol X_t^* 
    (\boldsymbol A_{\boldsymbol \gamma}^{*(k+1)})^{-1} 
    {\boldsymbol X_t^{*}}'
    ]^{-1}
    \boldsymbol X_t^* 
    (\boldsymbol A_{\boldsymbol \gamma}^{*(k+1)})^{-1},
\end{equation*}
to only invert an $n \times n$ matrix instead of a $p \times p$ matrix.
