# Supplementary material for: Bayesian method for causal inference in spatially-correlated multivariate time series
Source: arXiv:1801.06282 source file (2018-03-12)
Supplement: Supplementary file 4 [file appendix-C.tex]

\newpage
\section{Plots in Section \ref{sec-4.3}}
\label{app-C}

\subsection{Traceplots and inefficient factors plot}

\begin{figure}[!h]
\centering
   \includegraphics[width=12cm]{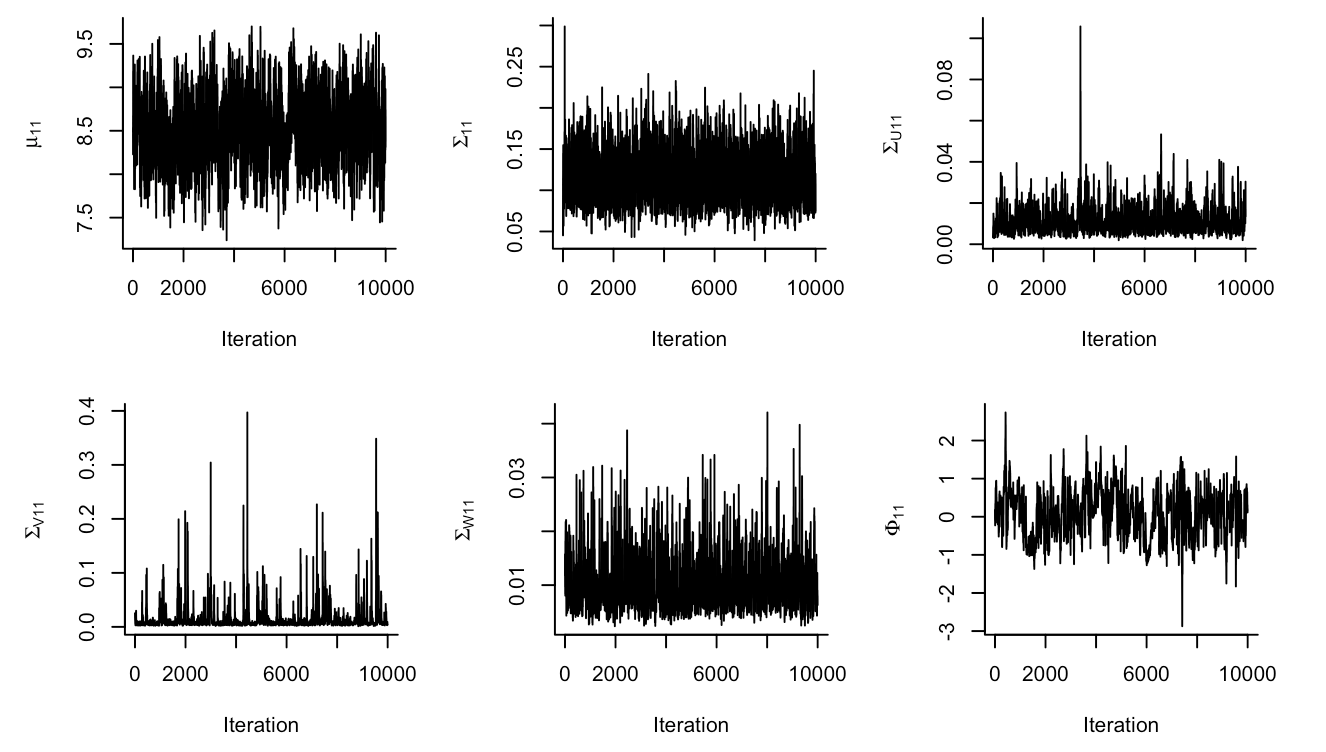}
   \caption{\small Traceplots for  
   $\boldsymbol \mu_{11}$, $\boldsymbol \Sigma_{11}$,
   $\boldsymbol \Sigma_{u 11}$, $\boldsymbol \Sigma_{v 11}$, 
   $\boldsymbol \Sigma_{w 11}$, $\boldsymbol \Phi_{11}$.}
   \label{fig-7}
\end{figure}

\bigskip

\begin{figure}[!h]
\centering
   \includegraphics[width=11cm]{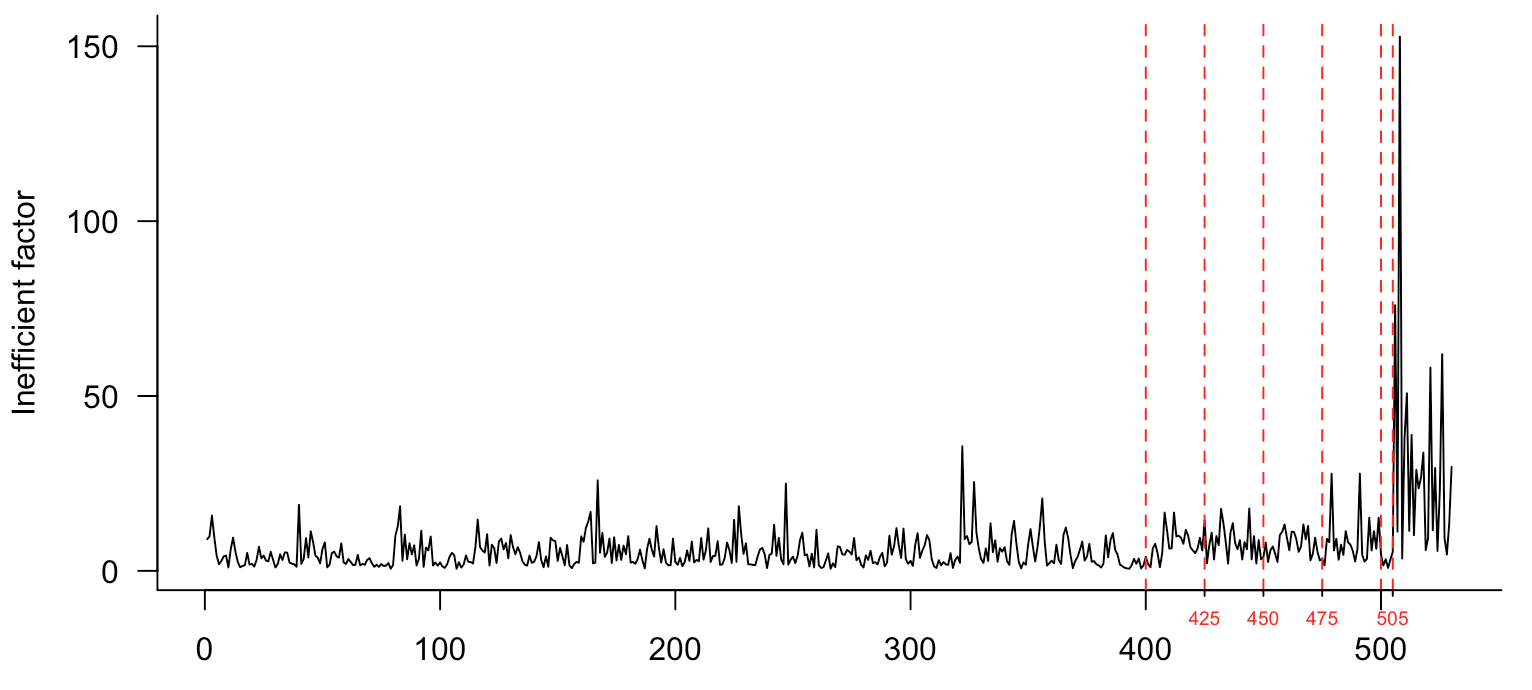}
   \caption{\small Plot of the inefficient factors (IFs) for
    $\boldsymbol \mu_{1:T}$, $\boldsymbol \Sigma$,
   $\boldsymbol \Sigma_{u}$, $\boldsymbol \Sigma_{v}$, 
   $\boldsymbol \Sigma_{w}$, 
   $\boldsymbol D$, $\boldsymbol \Phi$. 
   The first 400 values are IFs for parameters in $\boldsymbol \mu_{1:T}$ 
   (5 datasets each with 80 time periods),
   the following 100 values are IFs for parameters in $\boldsymbol \Sigma$,
   $\boldsymbol \Sigma_{u}$, $\boldsymbol \Sigma_{v}$, and
   $\boldsymbol \Sigma_{w}$, with each has 25 parameters,
   the next 5 values are IFs for parameters in $\boldsymbol D$;
   and the last 25 values are IFs for parameters in
   $\boldsymbol \Phi$.
   The red lines separate IFs result from different parameters.}
   \label{fig-8}
\end{figure}

\FloatBarrier

\newpage

\subsection{Plot of the results in the sensitivity study}

\begin{figure}[!h]
\centering
    \makebox[\textwidth][c]{\includegraphics[width=1.1\textwidth]{Paper-BA/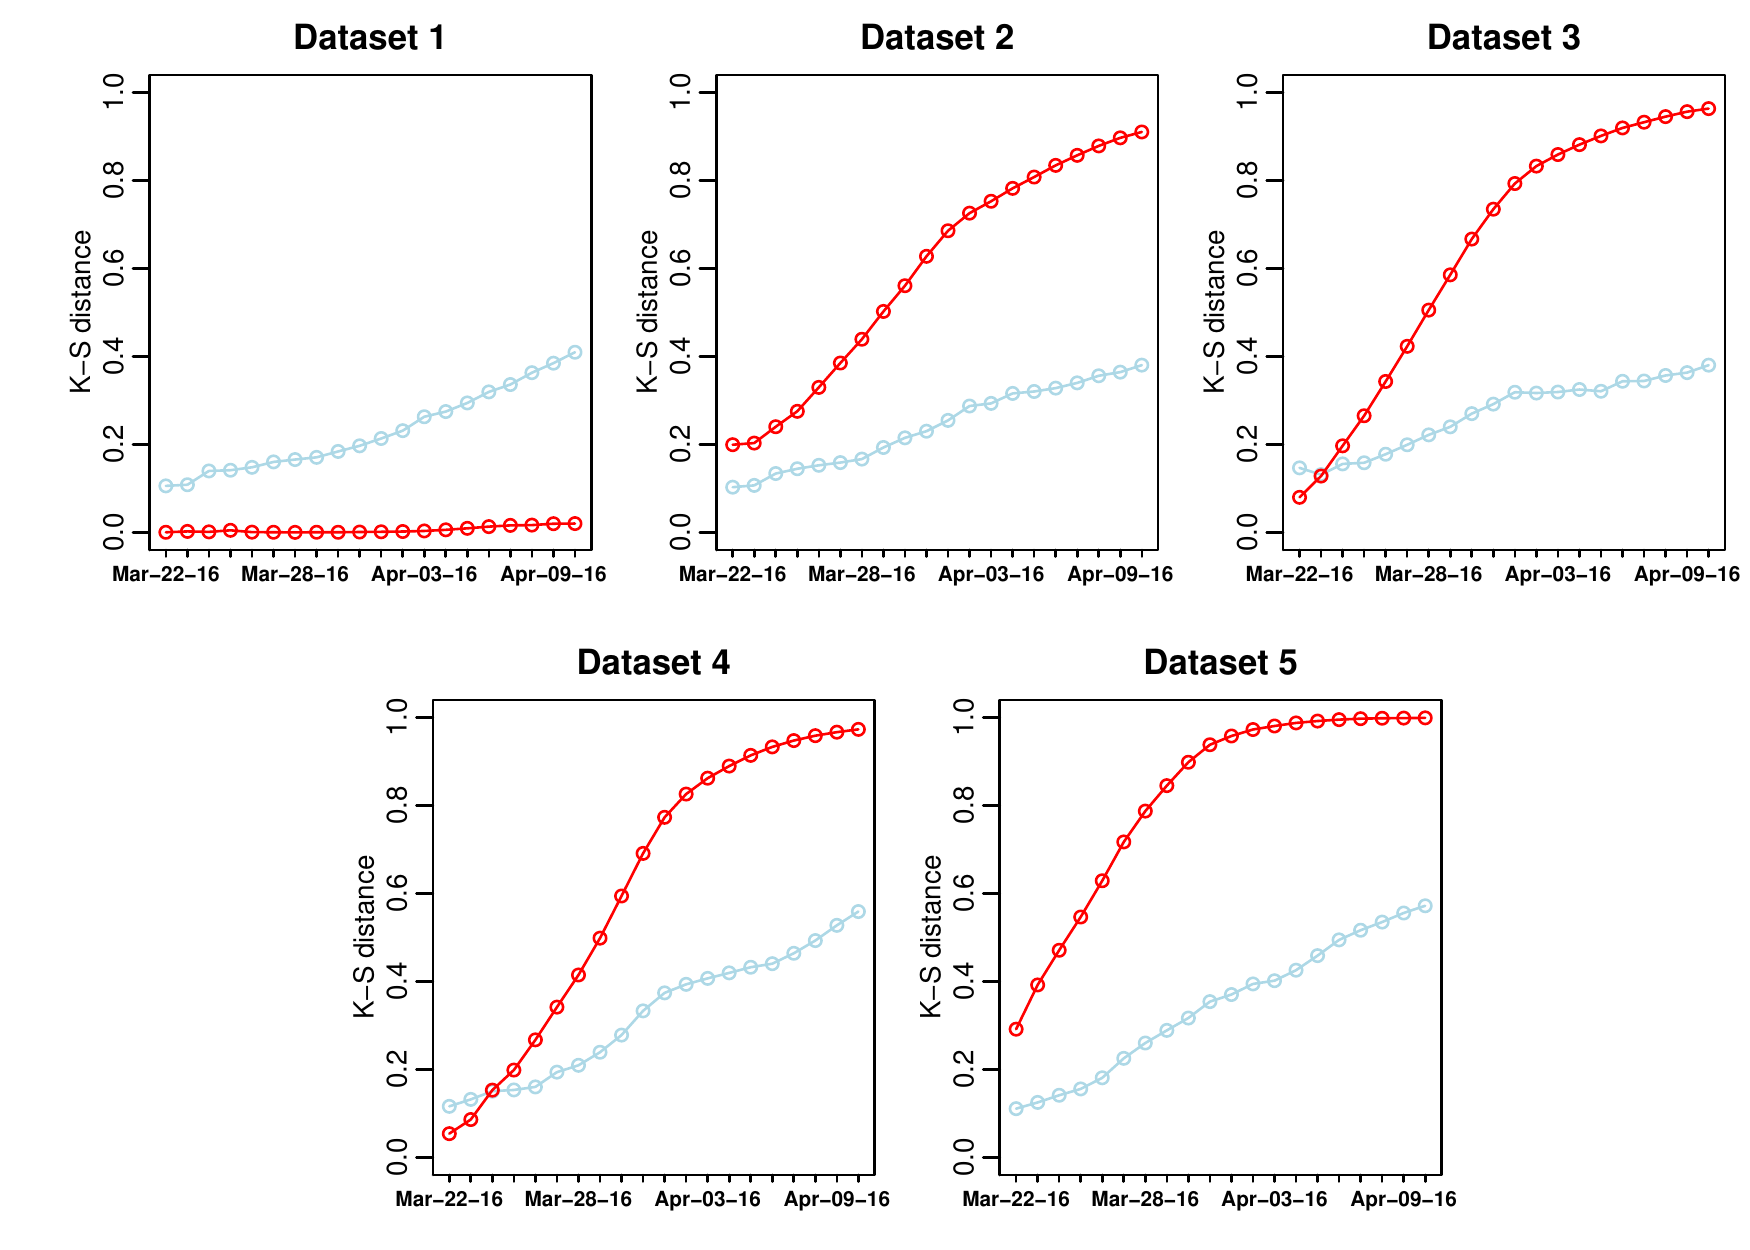}}
   \caption{\small 
   Results of applying the new method for detecting causal impacts in Dataset 1, $\dots$, Dataset 5 with the data generated from model (\ref{equ-5.4}) during the causal period from March, 22, 2016 to April, 9, 2016. In each subplot, the red line gives the one-sided KS distances between two posterior distributions with one is given the observed data and the other is given their corresponding counterfactuals; the light blue line gives the corresponding thresholds.}
   \label{fig-sensitivity}
\end{figure}

\FloatBarrier

\newpage 

\subsection{Plot of the results for choosing thresholds at the 99\% upper percentile}

\begin{figure}[!h]
\centering
    \makebox[\textwidth][c]{\includegraphics[width=1.1\textwidth]{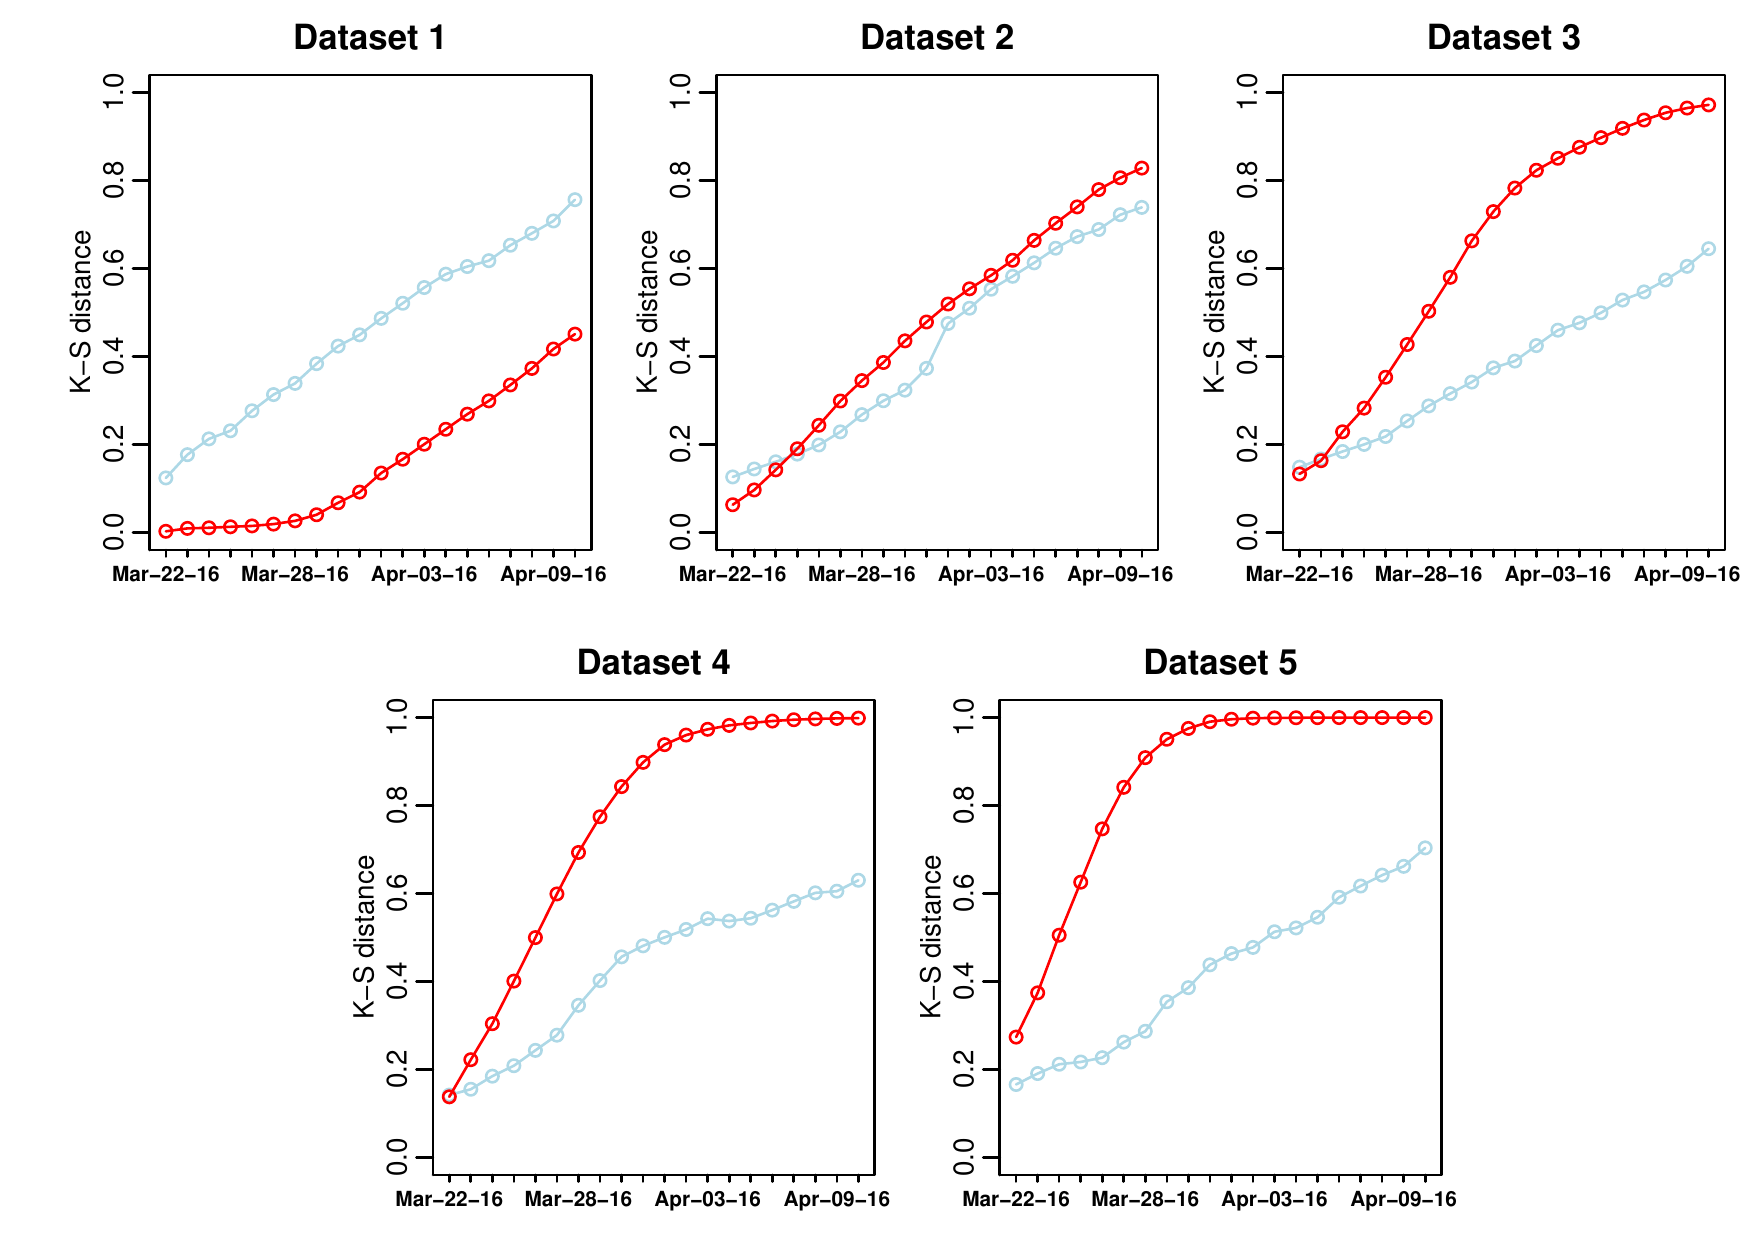}}
   \caption{\small 
   Results of applying the new method for detecting causal impacts in Dataset 1, $\dots$, Dataset 5 during the causal period from March, 22, 2016 to April, 9, 2016 with thresholds chosen as the 99\% upper percentile from the one-sided KS distances obtained from $30$ generated counterfactuals. 
   In each subplot, the red line gives the one-sided KS distances between two posterior distributions with one is given the observed data and the other is given their corresponding counterfactuals; the light blue line gives the corresponding thresholds.}
   \label{fig-ks-99}
\end{figure}

\FloatBarrier
